# Supplementary material for: RECAP: Retrieval-Enhanced Context-Aware Prefix Encoder for Personalized Dialogue Response Generation
Source: arXiv:2306.07206 source file (2023-06-12)
Supplement: Supplementary file 1 [file computation.tex]

\section{Computational Experiments Details}
\label{sec:computation}

% \begin{table}[!ht]
% \begin{adjustbox}{max width=\columnwidth}
% \begin{tabular}{lcc}
% \toprule
%                    & \# Params & Training Time (hr) \\ \midrule
% DialoGPT           & 124M      & 8                  \\
% DialoGPT + history & 124M      & 37                 \\
% DHAP               & 431M      & 25                 \\
% MSP                & 437M      & 15                 \\ \midrule
% RE                 & 198M      & 13                 \\
% CAP                & 269M      & 22                 \\ \bottomrule
% \end{tabular}
% \end{adjustbox}
% \caption{Total number of parameters and training time (on 2 \texttimes\ A40 GPUs) for all neural models.}
% \label{table:computation}
% \end{table}

\subsection{Neural Models}

All neural models used in this work are trained on 2 \texttimes\ A40 GPUs with half precision training. The total number of parameters and training time are shown in \autoref{table:computation}. For MSP, the numbers are sums over all sub-modules (i.e. three refiners and DialoGPT generator).

\subsection{Linear/Logistic Regression Models}
\label{sec:lr}

We train linear/logistic regression models with scikit-learn \cite{scikit-learn}\footnote{\url{https://scikit-learn.org/stable}} for personal traits evaluation.
Specifically, we train one linear regression model for age prediction and five logistic regression models for gender and MBTI prediction.
The input features are the most frequent 4,0000 TF-IDF weighted 1-3 word ngrams.
We use L-BFGS solver for the logistic regression models.
The best C value (i.e. inverse of regularization strength) for the gender and MBTI models are 10, 1, 10, 50, and 0.1, respectively.
All models can be trained within 20 seconds on a single CPU.
